# Supplementary material for: TFDM: Time-Variant Frequency-Based Point Cloud Diffusion with Mamba
Source: arXiv:2503.13004 source file (2025-03-17)
Supplement: Supplementary file 1 [file X_suppl.tex]

\clearpage
\setcounter{page}{1}
\maketitlesupplementary

% In this supplementary material, we first provide additional details on the methods presented in the main paper. Subsequentially, we provide the reference code implementation and our point cloud examples which achieve the state-of-the-art, validating our results. The code can be tested according to the README file in code documents. Finally, we provide further visualizations of our methods.

\noindent In this documentation, we supplement additional materials to support our findings, observations, and experimental results.
Specifically, it is organized as follows:
\begin{itemize}
    \item \cref{sec:visual} supplements further visualizations of our methods.
    \item \cref{sec:pre} provides additional details on the methods presented in the main paper.
    \item \cref{sec:ablation} gives full anaylysis of hyperparameters.
    \item \cref{sec:code} provides the reference code implementation (with README file) and our point cloud examples which achieve the state-of-the-art, validating our results.
\end{itemize}

\section{Visualization}
\label{sec:visual}

This section presents additional qualitative results of our generative models, as shown in Figure 1. Furthermore, a supplementary video is provided to demonstrate the generation outcomes (video.mp4) in greater detail. We also demonstrate more details in~\cref{fig:figure1}, our chair has a smoother back, and our car retains the rear-view mirror.

\section{Background}
\label{sec:pre}
In this section, we replenish more details of foundational concepts relate to our model.
\subsection{Denoising Diffusion Probabilistic Model}
\label{sec:1.1}
For given samples $x_0\sim q(x_{0})$, the diffusion model~\cite{ddpm_initial-idea,ddpm_first_2d} gradually reverses a Markovian fixed forward diffusion process:
\begin{align}
    q(\mathbf{x}_{1:T}|\mathbf{x}_0)&= \prod\nolimits_{t=1}^{T} q(\mathbf{x}_{t}|\mathbf{x}_{t-1}),\\
    q(\mathbf{x}_{t}|\mathbf{x}_{t-1}) &=\mathcal{N}({\mathbf{x}_{t}; \sqrt{\alpha_{t}}\mathbf{x}_{t-1}, (1-\alpha_{t})\mathbf{I}}),
\end{align}
where $T$ denotes the time step, $q(\mathbf{x}_{t}|\mathbf{x}_{t-1})$ is the transition kernel progressively perturbs the input with a sequence of pre-defined variance schedule $(1-\alpha_{1}),...,(1-\alpha_{T})$. 

The reverse process is parameterized as a Markovian chain $p_{\theta}(\mathbf{x}_{0:T})$ which is equal to $p(\mathbf{x}_{T})\prod\nolimits_{t=1}^{T} p_{\theta}(\mathbf{x}_{t-1}|\mathbf{x}_{t})$,
\begin{equation}
    p_{\theta}(\mathbf{x}_{t-1}|\mathbf{x}_{t}) = \mathcal{N}(\mathbf{x}_{t-1};{\mu}_\theta(\mathbf{x}_t,t),\sigma_t^2\mathbf{I}),
    \label{model_obj}
\end{equation}
where $p(\mathbf{x}_T)$ is standard Gaussian and ${\mu}_\theta(\mathbf{x}_t,t)$ is the learnable object, with setting $\sigma_t^2$ as a fixed variance schedule.  This object is optimized by matching the ground truth denoising step, which can be interpreted as learning the source noise  ${\epsilon}_0$ by minimizing $w\left(t\right)\parallel{{\mathbf{\epsilon}}}_\theta\left(x_t,t\right)-{\epsilon}_0\parallel_2^2$, where $w\left(t\right)$ is a parameter only depends on timestep. The optimization objective thus becomes:
\begin{equation}
    \mathcal{L} = \mathbb{E}_{t\sim [1,T]}w\left(t\right)\parallel{{\mathbf{\epsilon}}}_\theta\left(\mathbf{x}_{t},t\right)-{\epsilon}_0\parallel_2^2
    \label{loss}
\end{equation}
After training, generation can be achieved via the inverse chain by sampling from a standard Gaussian distribution.

\begin{figure}[t]
\begin{center}
\includegraphics[width=1\linewidth]{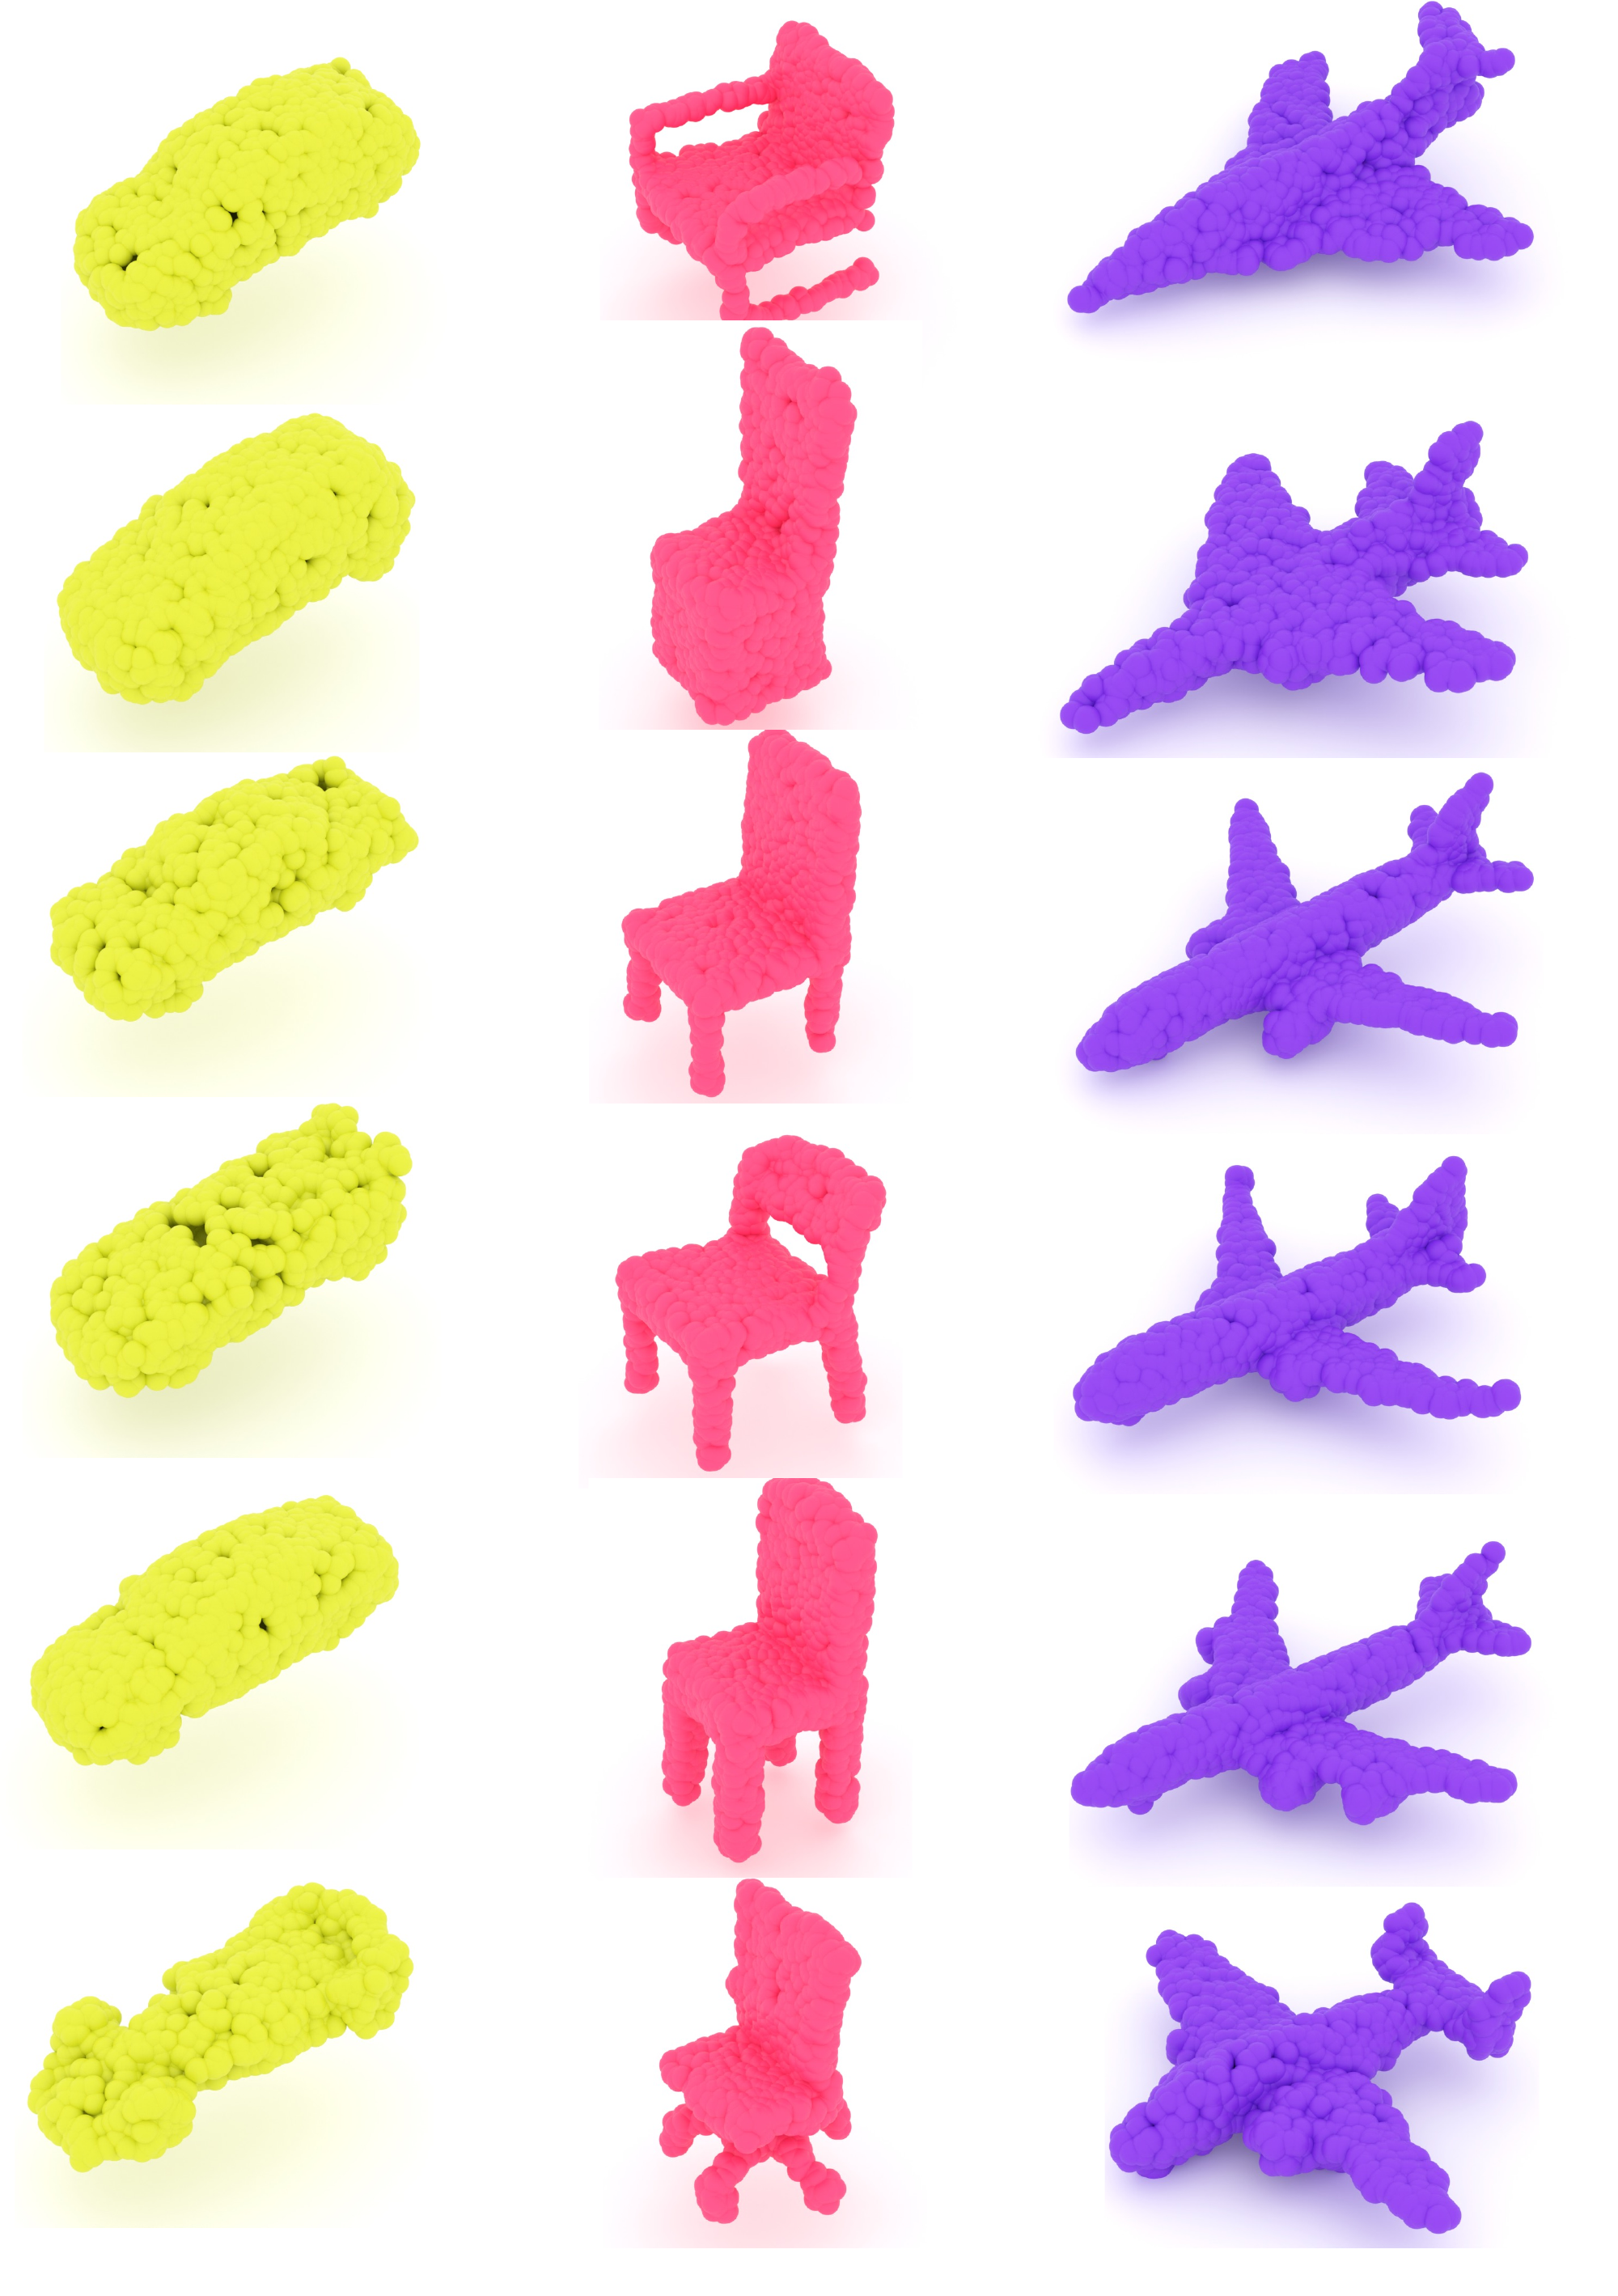} 
\end{center}
   \vspace{-5mm}
   \caption{More Qualitative Results}
   % \vspace{-6mm}
\label{fig:overview}
\end{figure}

\subsection{State Space Model}
\label{sec:1.2}
The State Space Model (SSM)~\cite{mamba_initial} can be described as a continuous system that maps a 1-D function or sequence $x(t)$ to $y(t)$ , with medilated through a N-D latent state $h(t)$.
\begin{equation}
    h^{'}(t) = \mathbf{A}h(t) + \mathbf{B}x(t), y(t) = \mathbf{C}h(t), 
\end{equation}
where $\mathbf{A},\mathbf{B}$ and $\mathbf{C}$ are parameters can be learned via gradient descent. 
Mamba~\cite{mamba_initial} improved the SSM by relaxing the time-invariance constraint and discretize the formulation via a timescable transformation parameter $\Delta$. By using zero-order hold techniques, the parameters can be defined as:
\begin{equation} 
  \label{eq:mamba}
  \overline{\mathbf{A}} = \exp(\Delta \mathbf{A}), \overline{\mathbf{B}} = (\Delta \mathbf{A})^{-1} \left( \exp(\Delta \mathbf{A}) - \mathbf{I} \right) \Delta \mathbf{B}. 
\end{equation}
Subsequently, \cref{eq:mamba} can be discretized and is able to compute the outputs as specific time step: 
\begin{equation}
    h^{'}(t) = \overline{\mathbf{A}}h(t) + \overline{\mathbf{C}}x(t), y(t) = \mathbf{C}h(t). 
\end{equation}
Finally, it employs a structured global convolution to enhance computational efficiency:
\begin{equation} 
   \overline{\mathbf{K}} = (\mathbf{C}\overline{\mathbf{B}},\ \mathbf{C}\overline{\mathbf{A}\mathbf{B}},\ \ldots,\ \mathbf{C}\overline{\mathbf{A}}^{M-1}\overline{\mathbf{B}}), \quad y = x * \overline{\mathbf{K}}, 
\end{equation}
where $M$ and $\overline{\mathbf{K}}$ represent individually the length of sequence x and the kernel of the global convolution.

\begin{figure}[t]
\begin{center}
\includegraphics[width=1\linewidth]{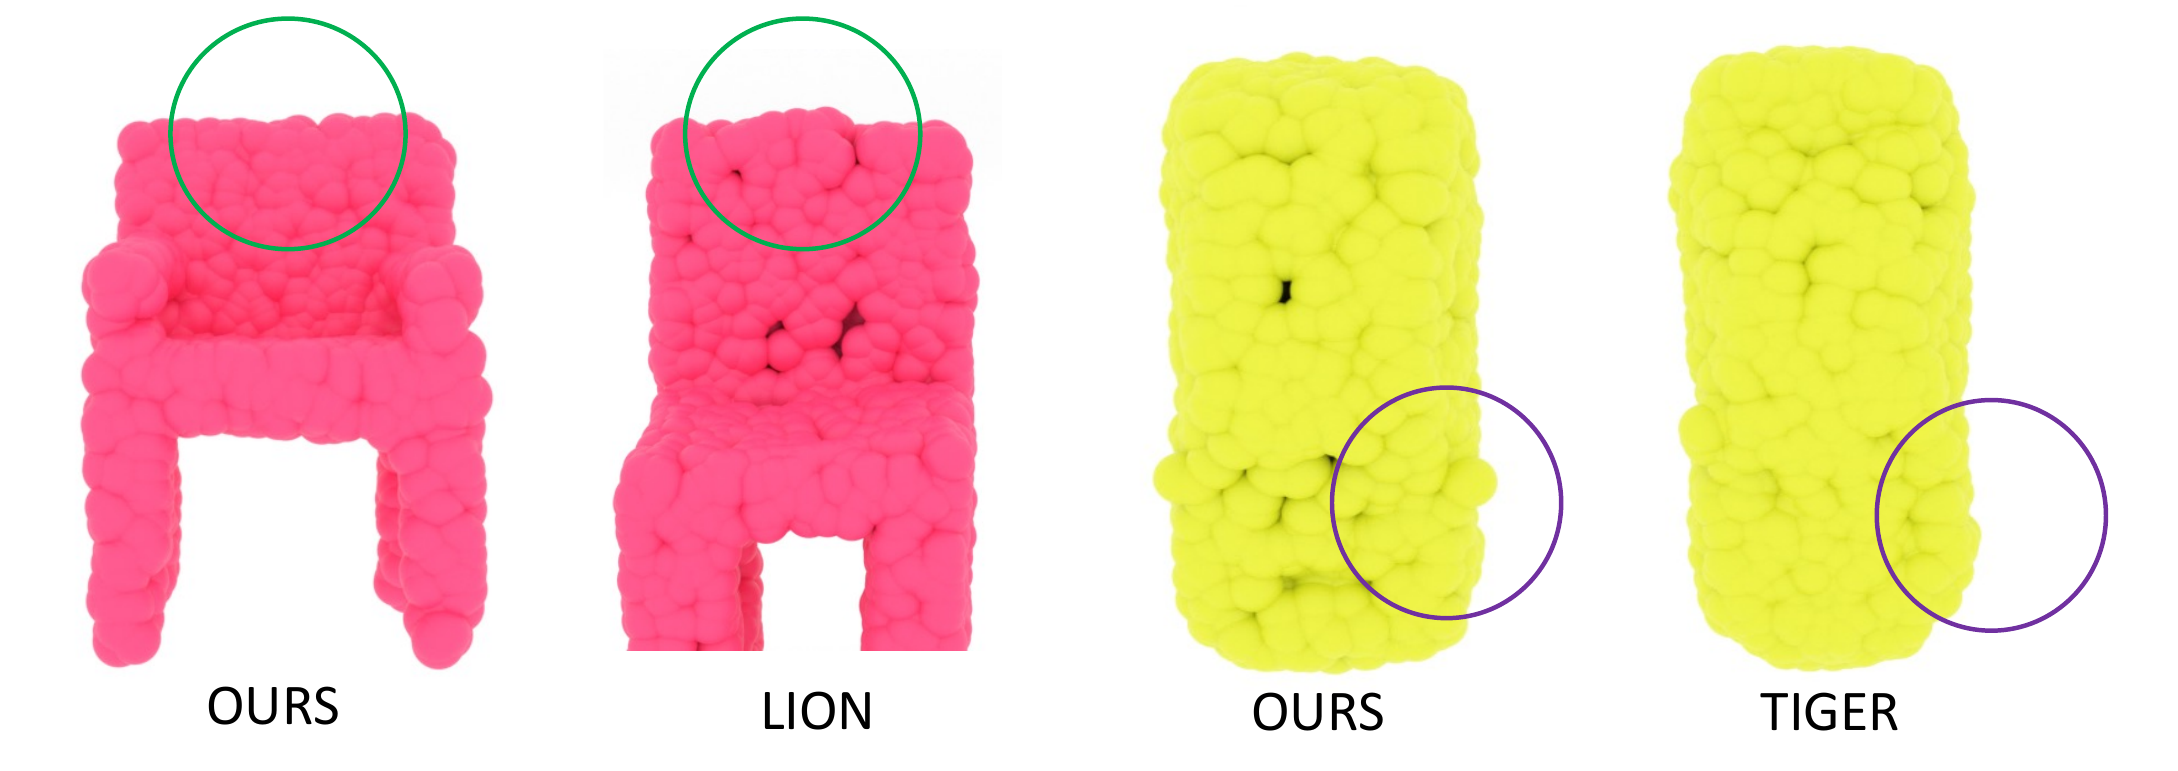}
% \framebox(220,40){}
\end{center}
   % \vspace{-6mm}
   % change:  solve the lower / higher value confused 
   \caption{Back of chair (Pink) - smooth(ours)/deformed(other) , Car side-view mirror (Yellow) - present(ours)/missing(other)}
   % \vspace{-6mm}
\label{fig:figure1}
% \vspace{-2mm}
\end{figure}

\subsection{Graph Filter}
\label{sec:1.3}
Given a graph $\mathcal{G} = (\mathcal{V},\mathbf{A},\mathbf{A}^u)$ let $\mathcal{V}= { v_1,...,v_N }$ denote a set of $N$ nodes and $\mathbf{A},\mathbf{A}^u \in \mathbb{R}^{N\times N}$ represent the weight and unweight adjacency matrix. We refer to one-channel features on all nodes to be a graph signal $\mathbf{s}\in \mathbb{R}^N$. $\mathbf{A}$ has eigen decomposition $\mathbf{A}=V\mathbf{\Lambda}V^{-1}$ where the matrix $V$
contains eigenvectors of $\mathbf{A}$ and $\mathbf{\Lambda}$ is diagonal eigenvalue matrix corresponding to ordered eigenvalues $\lambda_1,...,\lambda_N$. 

As stated in~\cite{garph_signal}, the ordered eigenvalues represent frequencies on the graph. Consider $\mathbf{A}$ as a graph shift operator and take a signal $\mathbf{s}$ to produce $\mathbf{y}= \mathbf{As}$, which is $V^{-1}\mathbf{y}=\mathbf{\Lambda}V^{-1}\mathbf{s} $. The graph Fourier transformation of graph signal $\mathbf{s}$ and $ \mathbf{y}$ :  $ \mathbf{\hat{s}}= V^{-1}\mathbf{s} ,\mathbf{\hat{y}}= V^{-1}\mathbf{y}$ could be considered as frequency contents of signal $\mathbf{s}$ and $\mathbf{y}$. Additionally, a graph filter is a polynomial in the graph shift~\cite{graph_signal2}: $h(\mathbf{A})=\sum_{l=0}^{L-1} h_{l}\mathbf{A}^l$, where 
$h_{l}, L $ denote filter coefficients and the length of filter respectively. This filter takes signal $\mathbf{s}$ and generate $\mathbf{y}=h(\mathbf{A})\mathbf{s} = Vh(\mathbf{\Lambda}V^{-1}\mathbf{s})$, making $V^{-1}\mathbf{y}=h(\mathbf{\Lambda}V^{-1}\mathbf{s})$ then $\mathbf{\hat{y}} =h(\mathbf{\Lambda} \mathbf{\hat{s}})$. The diagonal matrix $h(\mathbf{\Lambda})$ is the graph frequency response of the filter
$h(\mathbf{A})$ can be denoted $\hat{h}(\mathbf{A})$, and the frequency response of $\lambda_{i}$ is $\sum_{l=1}^{L-1}h_{l}\lambda_{i}^l$.

\section{Ablation Study of hyperparameters}
\label{sec:ablation}
In \cref{tab:table4}, we present hyperparameter analysis on the influence of $\tau$ and $\zeta$, where $\tau$ specifies the number of timesteps that utilize frequency information, and $\zeta$,indicates the percentage of the subsampling process that uses a high-pass filter. Setting $\tau=50$ and $\zeta=0.875$ achieves the best overall results (\cref{tab:table4}), although $\tau=75$ yields a slightly improved 1-NNA-Abs50 EMD, it also increases computational cost.

\begin{table}
% \footnotesize
\setlength{\tabcolsep}{10pt}
 \vspace{-3mm}
 \begin{center}
    \resizebox{.48\textwidth}{!}
    {\begin{tabular}{@{}lcc|cccc@{}}
    
    \hline 
       & $\tau$    & $\zeta$    & CD $\downarrow$  & EMD $\downarrow$ & CD  $\uparrow$  &  EMD $\uparrow$ \\
       &  &  &(1-NNA-Abs50)   &(1-NNA-Abs50)  & (Cov) & (Cov)\\
    \hline
       (a) & 10      &    0.875       & 4.41   & 2.43   &   49.26 &  52.43       \\
       (b) & 25       &      0.875       & 3.54   & 1.99   &   49.01 &  53.99       \\
       (c) & 50        &  0.875      & 3.25   &  1.68   &   49.84  &  54.98       \\
       (d) & 75     &   0.875        & 3.32   & 1.56   &   49.78 &  54.37      \\
       
       (e) & 50 &  0.75      & 4.15   & 2.37   & 48.93   &    53.46     \\
       (f) & 50     & 0.625      & 4.76  &  2.59  &   48.83 &  53.54      \\
       (g) & 50     & 0.5      & 4.91  &  3.01  &   48.12 &  52.94       \\
       
    \hline
    \end{tabular}}
    \end{center}
    \vspace{-6mm}
    \caption{Ablations on hyperparameters $\tau$ and $\zeta$ v.s. 1-NNA/Cov.}
    \label{tab:table4}
    \vspace{-4.5mm}
\end{table}

% \section{Details of Decoder}
% \notes{
% We provide the details of decoder, where shown in \cref{fig:decoder}. To upsample the latent point cloud back to the 3D space and predict the corresponding noise, we employ trilinear interpolation to convert the latent point cloud $\mathcal{\hat{X}}_{out}^{m} \in \mathbb{R}^{M \times D}$ with the accompanying coordinates, to $\mathcal{X}_t \in \mathbb{R}^{N \times 3}$. Similarly to \cref{sec:4.3}, we voxelize the $\mathcal{\hat{X}}_{out}^{m}$ into volume $\tilde{\boldsymbol{V}_{out}} \in \mathbb{R}^{L \times L\times L \times D}$ and \notes{following an additional 3D convolutional network while preserving the original shape,} then query use $\mathcal{X}_t$,  thereby obtaining the final prediction of the noise $\mathbf{\epsilon}_\theta$.
% }
% \begin{figure}[t]
% \begin{center}
% \includegraphics[width=1\linewidth]{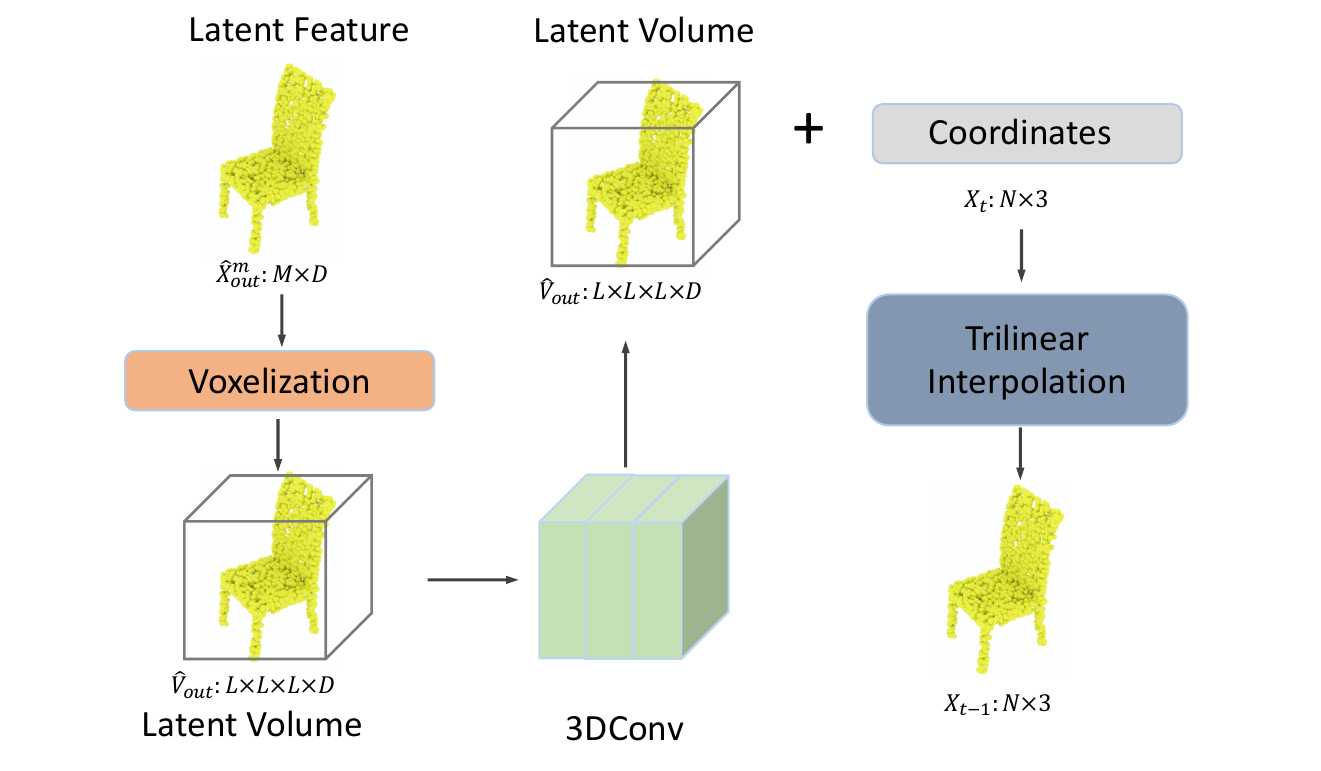} 
% \end{center}
%    % \vspace{-5mm}
%    \caption{The overview of decoder, the final prediction $X_{t-1}$ can be obtained by querying the latent volume $V_{out} $ with the coordinates $X_t$}
%    % \vspace{-6mm}
% \label{fig:decoder}
% \end{figure}

% \vspace{10pt}
\section{Code}
\label{sec:code}
We provide the reference code in the supplementary material. We will release the full source code once the paper is accepted. The code can be found in the designated folder (folder name: code). Additionally, we include sampled point cloud generated by our model for testing purposes (\cref{sec:1.6}). You could follow the steps:

\subsection{Dependency}
\begin{itemize}
%  \item Ubuntu 20.04
  \item Python 3.8
  \item CUDA 11.6
  \item Pytorch 1.12.1 + cu116
\end{itemize}

\subsection{Environment}
Can simply install via:
\begin{lstlisting}[language=bash, caption={Install Environment}]
conda env create -f ldm.yml
conda activate ldm
\end{lstlisting}

\subsection{Compile}
\begin{lstlisting}[language=bash, caption={Compilation Steps}]
export TORCH_CUDA_ARCH_LIST="6.1;6.2;7.0;7.5;8.0;8.6"
cd metrics/PyTorchEMD
python setup.py install
cp build/lib.linux-x86_64-3.8/emd_cuda.cpython-36m-x86_64-linux-gnu.so .
\end{lstlisting}

\subsection{Dataset}
Download the ShapeNet Dataset~\cite{chang2015shapenet}:
\begin{lstlisting}[language=bash, caption={Download Dataset}]
gdown https://drive.google.com/uc?id=1sw9gdk_igiyyt7MqALyxZhRrtPvAn0sX
unzip ShapeNetCore.v2.PC15k.zip
\end{lstlisting}

\subsection{Training \& Testing}
\begin{lstlisting}[language=bash, caption={Training and Testing}]
python train_generation.py --category chair --bs 32 --mamba_depth 8 --latent_size 512 --order 'hilbert' --use_multi_order True
python test_generation.py --category chair --mamba_depth 8 --latent_size 512 --order 'hilbert' --use_multi_order True --model 'saved_checkpoint_path'
\end{lstlisting}

\subsection{Evaluation}
We provide the generated point cloud set which achieve the state-of-the-art results:
\label{sec:1.6}
\begin{lstlisting}[language=bash, caption={Evaluation}]
python test.py --category car --eval_path 'Best_Save_points/best_car_cd_cov.pth'
\end{lstlisting}

\noindent
Further details can be found in README file.
